# Supplementary material for: TouchUp-G: Improving Feature Representation through Graph-Centric Finetuning
Source: arXiv:2309.13885 source file (2025-03-30)
Supplement: Supplementary file 1 [file 099appendix.tex]

\subsection{Experimental Details}
\label{sec:exp-details}
\paragraph{Dataset Construction}
For node classification, we follow the split and evaluation in~\cite{hu2020open}. For link prediction, since we are using new datasets and no public split is available, we do random split on \ogbproducts, \books, \amazoncp. \ogbproducts ~and \books ~are splitted at a ratio of 60$\%$/10$\%$/30$\%$. \amazoncp ~is using a 80$\%$/10$\%$/10$\%$ split ratio. For every validation and test edges, we randomly generate 1000 negatives for \books ~dataset, 100 negatives for \ogbproducts ~and 300 negatives for \amazoncp. All of these graphs are homogeneous, undirected graphs. The dataset construction pipelines for \books ~and \amazoncp ~dataset will be made public upon acceptance in a notebook, so that others can construct the same dataset following the steps. 

\paragraph{Hyperparameter Tuning}
For PMs, we conduct extensive hyperparameter tuning using grid search. We search on the learning rates $ = \{$1e-1, 1e-2, 1e-3, 1e-4, 5e-4, 5e-5$\}$. The training batch size is set to 64 for all datasets. We use gradient clipping and early stopping to prevent overfitting on the training edges~\cite{li2020gradient, smith2021origin}
We used four Nvidia A40 GPU to train the model. Due to the fact that validating on the full validation split for one epoch is extremely time-consuming, we subsample a small set from the full validation test (1$\%$ of the edges in the validation set), and use MRR over 5 negative examples to select the best checkpoint. The touchup model weights from the best performing epoch are then used to generate the finetuned feature embeddings. 

For GNNs, we also do grid search of hyperparameters.
We search on the learning rates $ = \{$1e-1, 1e-2, 1e-3, 1e-4, 5e-4, 1e-4, 5e-5$\}$ and the number of layers $= \{1,2,3\}$. The training batch size and hidden dimension is set to 512 for all datasets. 
For GATv2, the number of heads is 8. We first do a grid search on the best performing hyperparameters before any touch-up. After touch-up, we use the same best performing hyperparameters.  
We used one Nvidia v100 GPU to train the model and repeat our experiments with three different random seeds. The test results are reported on the epoch with the best validation performance.
